# Supplementary material for: Federated Learning via Plurality Vote
Source: arXiv:2110.02998 source file (2022-12-10)
Supplement: Supplementary file 2 [file voting_methods.tex]

\section{Voting Methods}

We review the definitions of several voting methods \citep{zhou2019ensemble}.  
Suppose we have a set of $M$ individual voters and $C$ candidate output labels $\{\psi_{1},\dots,\psi_{C}\}$.   
For the $m$th voter, it will output result $\votevec_{m} = [v_{m,1},\, \dots, v_{m,C}]^\top$. 
Here, the $i$th entry $v_{m,i} \in \{0,\,1\}$, which takes the value one if the voter chooses the candidate $\psi_{i}$ and zero otherwise. 

\emph{Majority vote} requires the winner to receive more than half of the votes; if none of the candidates receives more than half of the votes, a rejection option will be given. 
The majority vote result can be written as 
\begin{equation}
\Psi_{\textrm{majority}} = \left\{ 
\begin{array}{l @{\;} l}
    \psi_{i},          & \textrm{ if }\displaystyle \sum_{m=1}^M v_{m,i} > \frac{1}{2} \sum_{j=1}^{C} \sum_{m=1}^M v_{m,j}, \\[3pt]
    \textrm{rejection},  & \textrm{otherwise}. 
\end{array}\right.
\end{equation}
\emph{Plurality vote} takes the class label that receives the largest number of votes as the final winner, i.e., 
\begin{equation}
    \Psi_{\textrm{plurality}} = \psi_{\argmax_{i} \sum_{m=1}^{M} v_{m,i}}.
\end{equation}
In the binary case with $C=2$, plurality vote resembles majority vote except that it does not have a rejection option. 
If more than two candidates receive the same number of votes, we randomly select one of them as the final results. 
\emph{Weighted vote} assigns different weights for voters and the result can be written as 
\begin{equation}
    \Psi_{\textrm{weighted}} = \psi_{\argmax_{i} \sum_{m=1}^{M} \lambda_m v_{m,i}},
\end{equation}
where $\lambda_{m}$ is the weight assigned to the $m$th voter. 
In contrast to the aforementioned vote methods, \emph{soft vote} produces the probability output. 
The probability that the $i$th candidate wins is calculated as 
\begin{equation}
    \widehat{\prob} (\Psi_{\text{soft}} = \psi_{i}) = \frac{1}{M} \sum_{m=1}^M  v_{m,i}. 
\end{equation}
