# Supplementary material for: Federated Learning via Plurality Vote
Source: arXiv:2110.02998 source file (2022-12-10)
Supplement: Supplementary file 3 [file algorithm.tex]

\section{FedVote ALgorithm}\label{appendix:algorithm}

We summarize the proposed FedVote method and its Byzantine-resilient variant in \paperalg{alg:fedvote}. 
When there are no attackers involved, we use \texttt{Option I}.
When we require the resilience against Byzantine failure, we choose \texttt{Option II}.
